# Supplementary material for: Ground- and Excited-State Dipole Moments and Oscillator Strengths of Full Configuration Interaction Quality
Source: arXiv:2211.04120 source file (2022-12-22)
Supplement: Supplementary file 1 [file supp_inf_dipole_cipsi.pdf]

# Supporting Information for "Ground- and Excited-State Dipole Moments and Oscillator Strengths of Full Configuration Interaction Quality"


Yann Damour,[1, a)] Raúl Quintero-Monsebaiz,[1] Michel Caffarel,[1] Denis Jacquemin,[2,3] Fábris Kossoski,[1] Anthony Scemama,[1] and Pierre-François Loos[1, b)]

[1)] *Laboratoire de Chimie et Physique Quantiques (UMR 5626), Université de Toulouse, CNRS, UPS, France*

[2)] *Nantes Université, CNRS, CEISAM UMR 6230, F-44000 Nantes, France*

[3)] *Institut Universitaire de France (IUF), F-75005 Paris, France*

[a)] Electronic mail: yann.damour@irsamc.ups-tlse.fr

[b)] Electronic mail: loos@irsamc.ups-tlse.fr

TABLE I. Dipole moments, excitation energies, and oscillator strengths in the length (L), velocity (V), and mixed (LV) representation for BH at the CC and SCI levels computed in various basis sets. An estimate of the exFCI extrapolation error is reported in parentheses.

| | | $^1\Sigma^+$ | $^1\Pi$(Val) | | | | |
|---|---|---|---|---|---|---|---|
| Basis | Method | $\lVert\boldsymbol{\mu}^{\text{GS}}\rVert$ (D) | $\Delta E_{\text{vert}}$ (eV) | $f^{\text{L}}$ | $f^{\text{V}}$ | $f^{\text{LV}}$ | $\lVert\boldsymbol{\mu}^{\text{ES}}\rVert$ (D) |
| aug-cc-pVDZ | CCSD | 1.389 | 2.970 | 0.051 | | | 0.530 |
| | CCSDT | 1.371 | 2.946 | 0.049 | | | 0.543 |
| | CCSDTQ | 1.370 | 2.947 | 0.049 | | | 0.545 |
| | CCSDTQP | 1.370 | 2.947 | 0.049 | | | 0.545 |
| | CIPSI | 1.370 | 2.947 | 0.049 | 0.062 | 0.055 | 0.542 |
| | exFCI | 1.370(0) | 2.947(0) | 0.049(0) | 0.062(0) | 0.055(0) | 0.542(0) |
| aug-cc-pVTZ | CCSD | 1.433 | 2.928 | 0.050 | | | 0.550 |
| | CCSDT | 1.410 | 2.900 | 0.048 | | | 0.558 |
| | CCSDTQ | 1.409 | 2.901 | 0.048 | | | 0.559 |
| | CIPSI | 1.408 | 2.901 | 0.048 | 0.057 | 0.052 | 0.554 |
| | exFCI | 1.408(0) | 2.901(0) | 0.048(0) | 0.057(0) | 0.052(0) | 0.554(0) |
| aug-cc-pVQZ | CCSD | 1.440 | 2.918 | 0.050 | | | 0.555 |
| | CCSDT | 1.416 | 2.890 | 0.048 | | | 0.561 |
| | CIPSI | 1.414 | 2.891 | 0.048 | 0.056 | 0.052 | 0.556 |
| | exFCI | 1.414(0) | 2.891(0) | 0.048(0) | 0.056(0) | 0.052(0) | 0.556(0) |
| aug-cc-pV5Z | CCSD | 1.443 | 2.915 | 0.050 | | | 0.556 |
| | CIPSI | 1.417 | 2.888 | 0.048 | 0.056 | 0.052 | 0.557 |
| | exFCI | 1.417(0) | 2.888(0) | 0.048(0) | 0.056(0) | 0.052(0) | 0.557(0) |

TABLE II. Dipole moments, excitation energies, and oscillator strengths in the length (L), velocity (V), and mixed (LV) representation for HCl at the CC and SCI levels computed in various basis sets. An estimate of the exFCI extrapolation error is reported in parentheses.

| | | $^1\Sigma^+$ | $^1\Pi$(Val) | | | | |
|---|---|---|---|---|---|---|---|
| Basis | Method | $\lVert\boldsymbol{\mu}^{\text{GS}}\rVert$ (D) | $\Delta E_{\text{vert}}$ (eV) | $f^{\text{L}}$ | $f^{\text{V}}$ | $f^{\text{LV}}$ | $\lVert\boldsymbol{\mu}^{\text{ES}}\rVert$ (D) |
| aug-cc-pVDZ | CCSD | 1.147 | 7.862 | 0.066 | | | 2.773 |
| | CCSDT | 1.131 | 7.814 | 0.065 | | | 2.745 |
| | CCSDTQ | 1.130 | 7.822 | 0.065 | | | 2.728 |
| | CCSDTQP | 1.130 | 7.823 | 0.065 | | | 2.727 |
| | CIPSI | 1.130 | 7.823 | 0.065 | 0.064 | 0.064 | 2.727 |
| | exFCI | 1.130(0) | 7.823(0) | 0.065(0) | 0.064(0) | 0.064(0) | 2.727(0) |
| aug-cc-pVTZ | CCSD | 1.097 | 7.906 | 0.056 | | | 2.526 |
| | CCSDT | 1.085 | 7.834 | 0.055 | | | 2.515 |
| | CCSDTQ | 1.084 | 7.837 | 0.055 | | | 2.502 |
| | CIPSI | 1.085 | 7.837 | 0.054 | 0.054 | 0.054 | 2.501 |
| | exFCI | 1.084(0) | 7.837(0) | 0.055(1) | 0.054(0) | 0.054(0) | 2.501(0) |
| aug-cc-pVQZ | CCSD | 1.111 | 7.954 | 0.051 | | | 2.410 |
| | CCSDT | 1.098 | 7.880 | 0.050 | | | 2.410 |
| | CIPSI | 1.099 | 7.882 | 0.050 | 0.049 | 0.049 | 2.409 |
| | exFCI | 1.097(1) | 7.882(0) | 0.050(0) | 0.049(0) | 0.050(0) | 2.398(4) |

TABLE III. Dipole moments, excitation energies, and oscillator strengths in the length (L), velocity (V), and mixed (LV) representation for $H_2O$ at the CC and SCI levels computed in various basis sets. An estimate of the exFCI extrapolation error is reported in parentheses.

| | | $^1A_1$ | $^1B_1$ (Ryd, $n \to 3p$) | | | | | $^1A_2$ (Ryd, $n \to 3p$) | | $^1A_1$ (Ryd, $n \to 3s$) | | | | |
|---|---|---|---|---|---|---|---|---|---|---|---|---|---|---|
| Basis | Method | $\Vert\boldsymbol{\mu}^{\text{GS}}\Vert$ (D) | $\Delta E_{\text{vert}}$ (eV) | $f^{\text{L}}$ | $f^{\text{V}}$ | $f^{\text{LV}}$ | $\Vert\boldsymbol{\mu}^{\text{ES}}\Vert$ (D) | $\Delta E_{\text{vert}}$ (eV) | $\Vert\boldsymbol{\mu}^{\text{ES}}\Vert$ (D) | $\Delta E_{\text{vert}}$ (eV) | $f^{\text{L}}$ | $f^{\text{V}}$ | $f^{\text{LV}}$ | $\Vert\boldsymbol{\mu}^{\text{ES}}\Vert$ (D) |
| aug-cc-pVDZ | CCSD | 1.870 | 7.447 | 0.057 | | | 1.404 | 9.213 | 0.936 | 9.861 | 0.103 | | | 1.095 |
| | CCSDT | 1.849 | 7.497 | 0.058 | | | 1.420 | 9.279 | 0.978 | 9.903 | 0.104 | | | 1.149 |
| | CCSDTQ | 1.848 | 7.529 | 0.058 | | | 1.415 | 9.313 | 0.974 | 9.937 | 0.105 | | | 1.143 |
| | CCSDTQP | 1.848 | 7.522 | 0.058 | | | 1.414 | 9.318 | 0.972 | 9.941 | 0.105 | | | 1.141 |
| | CIPSI | 1.848 | 7.533 | 0.058 | 0.059 | 0.059 | 1.414 | 9.318 | 0.972 | 9.941 | 0.105 | 0.103 | 0.104 | 1.141 |
| | exFCI | 1.848(0) | 7.532(0) | 0.058(0) | 0.059(0) | 0.059(0) | 1.414(0) | 9.318(0) | 0.972(0) | 9.941(0) | 0.105(0) | 0.103(0) | 0.104(0) | 1.141(0) |
| aug-cc-pVTZ | CCSD | 1.864 | 7.596 | 0.053 | | | 1.549 | 9.361 | 1.056 | 9.957 | 0.098 | | | 1.163 |
| | CCSDT | 1.842 | 7.591 | 0.054 | | | 1.565 | 9.368 | 1.110 | 9.949 | 0.100 | | | 1.221 |
| | CCSDTQ | 1.840 | 7.620 | 0.054 | | | 1.559 | 9.400 | 1.107 | 9.981 | 0.100 | | | 1.215 |
| | CIPSI | 1.840 | 7.624 | 0.054 | 0.056 | 0.055 | 1.558 | 9.405 | 1.105 | 9.986 | 0.100 | 0.102 | 0.101 | 1.214 |
| | exFCI | 1.840(0) | 7.624(0) | 0.054(0) | 0.056(0) | 0.055(0) | 1.557(1) | 9.405(0) | 1.105(1) | 9.986(0) | 0.100(0) | 0.102(0) | 0.101(0) | 1.214(1) |
| aug-cc-pVQZ | CCSD | 1.873 | 7.660 | 0.052 | | | 1.655 | 9.422 | 1.237 | 10.004 | 0.095 | | | 1.226 |
| | CCSDT | 1.850 | 7.637 | 0.053 | | | 1.667 | 9.410 | 1.294 | 9.979 | 0.097 | | | 1.286 |
| | CIPSI | 1.849 | 7.668 | 0.053 | 0.054 | 0.053 | 1.666 | 9.444 | 1.282 | 10.015 | 0.097 | 0.099 | 0.098 | 1.284 |
| | exFCI | 1.848(0) | 7.669(0) | 0.053(0) | 0.054(0) | 0.054(0) | 1.659(2) | 9.446(0) | 1.289(2) | 10.015(1) | 0.097(0) | 0.099(0) | 0.098(0) | 1.278(1) |

TABLE IV. Dipole moments, excitation energies, and oscillator strengths in the length (L), velocity (V), and mixed (LV) representation for $H_2S$ at the CC and SCI levels computed in various basis sets. An estimate of the exFCI extrapolation error is reported in parentheses.

| | | $^1A_1$ | $^1A_2$ (Ryd, $n \to 4p$) | | $^1B_1$ (Ryd, $n \to 4s$) | | | | |
|---|---|---|---|---|---|---|---|---|---|
| Basis | Method | $\|\boldsymbol{\mu}^{\text{GS}}\|$ (D) | $\Delta E_{\text{vert}}$ (eV) | $\|\boldsymbol{\mu}^{\text{ES}}\|$ (D) | $\Delta E_{\text{vert}}$ (eV) | $f^{\text{L}}$ | $f^{\text{V}}$ | $f^{\text{LV}}$ | $\|\boldsymbol{\mu}^{\text{ES}}\|$ (D) |
| aug-cc-pVDZ | CCSD | 1.031 | 6.343 | 0.113 | 6.141 | 0.068 | | | 1.983 |
| | CCSDT | 1.016 | 6.286 | 0.131 | 6.098 | 0.067 | | | 1.946 |
| | CCSDTQ | 1.015 | 6.286 | 0.137 | 6.103 | 0.067 | | | 1.934 |
| | CCSDTQP | 1.015 | 6.286 | 0.137 | 6.103 | 0.067 | | | 1.933 |
| | CIPSI | 1.016 | 6.286 | 0.138 | 6.103 | 0.067 | 0.067 | 0.067 | 1.934 |
| | exFCI | 1.016(1) | 6.286(0) | 0.137(1) | 6.103(0) | 0.067(0) | 0.067(0) | 0.067(0) | 1.934(1) |
| aug-cc-pVTZ | CCSD | 0.990 | 6.246 | 0.503 | 6.295 | 0.064 | | | 1.893 |
| | CCSDT | 0.978 | 6.185 | 0.496 | 6.237 | 0.063 | | | 1.875 |
| | CCSDTQ | 0.977 | 6.181 | 0.498 | 6.238 | 0.063 | | | 1.866 |
| | CIPSI | 0.977 | 6.181 | 0.503 | 6.238 | 0.063 | 0.063 | 0.063 | 1.873 |
| | exFCI | 0.977(0) | 6.181(0) | 0.499(1) | 6.238(0) | 0.063(0) | 0.063(0) | 0.063(0) | 1.866(1) |
| aug-cc-pVQZ | CCSD | 1.001 | 6.212 | 0.650 | 6.348 | 0.062 | | | 1.822 |
| | CCSDT | 0.990 | 6.153 | 0.636 | 6.288 | 0.061 | | | 1.815 |
| | CIPSI | 0.989 | 6.139 | 0.647 | 6.279 | 0.061 | 0.061 | 0.061 | 1.831 |
| | exFCI | 0.989(1) | 6.147(3) | 0.637(0) | 6.287(0) | 0.061(1) | 0.061(0) | 0.061(0) | 1.812(9) |

TABLE V. Dipole moments, excitation energies, and oscillator strengths in the length (L), velocity (V), and mixed (LV) representation for BF at the CC and SCI levels computed in various basis sets. An estimate of the exFCI extrapolation error is reported in parentheses.

| | | $^1A_1$ | $^1\Pi$ (Val, $\sigma \to \pi^*$) | | | | |
|---|---|---|---|---|---|---|---|
| Basis | Method | $\|\boldsymbol{\mu}^{\text{GS}}\|$ (D) | $\Delta E_{\text{vert}}$ (eV) | $f^{\text{L}}$ | $f^{\text{V}}$ | $f^{\text{LV}}$ | $\|\boldsymbol{\mu}^{\text{ES}}\|$ (D) |
| aug-cc-pVDZ | CCSD | 0.832 | 6.534 | 0.479 | | | 0.240 |
| | CCSDT | 0.861 | 6.491 | 0.475 | | | 0.311 |
| | CCSDTQ | 0.861 | 6.486 | 0.474 | | | 0.316 |
| | CCSDTQP | 0.860 | 6.485 | 0.474 | | | 0.316 |
| | CIPSI | 0.860 | 6.485 | 0.474 | 0.500 | 0.487 | 0.312 |
| | exFCI | 0.860(0) | 6.485(0) | 0.474(0) | 0.500(0) | 0.487(0) | 0.312(0) |
| aug-cc-pVTZ | CCSD | 0.794 | 6.464 | 0.475 | | | 0.222 |
| | CCSDT | 0.824 | 6.423 | 0.469 | | | 0.293 |
| | CCSDTQ | 0.824 | 6.417 | 0.468 | | | 0.300 |
| | CIPSI | 0.826 | 6.417 | 0.468 | 0.491 | 0.480 | 0.292 |
| | exFCI | 0.824(1) | 6.417(0) | 0.468(0) | 0.490(1) | 0.479(0) | 0.294(1) |
| aug-cc-pVQZ | CCSD | 0.783 | 6.449 | 0.475 | | | 0.207 |
| | CCSDT | 0.812 | 6.410 | 0.468 | | | 0.279 |
| | CIPSI | 0.817 | 6.404 | 0.468 | 0.491 | 0.479 | 0.278 |
| | exFCI | 0.813(3) | 6.403(1) | 0.468(0) | 0.489(1) | 0.478(1) | 0.282(2) |

TABLE VI. Dipole moments, excitation energies, and oscillator strengths in the length (L), velocity (V), and mixed (LV) representation for CO at the CC and SCI levels computed in various basis sets. An estimate of the exFCI extrapolation error is reported in parentheses.

| | | $^1A_1$ | $^1\Pi$ (Val, $\sigma \to \pi^*$) | | | | |
|---|---|---|---|---|---|---|---|
| Basis | Method | $\lVert\boldsymbol{\mu}^{\text{GS}}\rVert$ (D) | $\Delta E_{\text{vert}}$ (eV) | $f^{\text{L}}$ | $f^{\text{V}}$ | $f^{\text{LV}}$ | $\lVert\boldsymbol{\mu}^{\text{ES}}\rVert$ (D) |
| aug-cc-pVDZ | CCSD | 0.078 | 8.671 | 0.167 | | | 0.157 |
| | CCSDT | 0.121 | 8.574 | 0.173 | | | 0.079 |
| | CCSDTQ | 0.130 | 8.563 | 0.174 | | | 0.072 |
| | CCSDTQP | 0.132 | 8.561 | 0.175 | | | 0.069 |
| | CIPSI | 0.133 | 8.560 | 0.175 | 0.185 | 0.180 | 0.071 |
| | exFCI | 0.132(0) | 8.560(0) | 0.175(0) | 0.184(0) | 0.179(0) | 0.070(0) |
| aug-cc-pVTZ | CCSD | 0.051 | 8.587 | 0.161 | | | 0.227 |
| | CCSDT | 0.104 | 8.492 | 0.164 | | | 0.137 |
| | CCSDTQ | 0.113 | 8.480 | 0.166 | | | 0.129 |
| | CIPSI | 0.117 | 8.476 | 0.166 | 0.174 | 0.170 | 0.134 |
| | exFCI | 0.116(1) | 8.477(0) | 0.166(0) | 0.173(0) | 0.169(1) | 0.129(1) |
| aug-cc-pVQZ | CCSD | 0.039 | 8.574 | 0.160 | | | 0.264 |
| | CCSDT | 0.094 | 8.480 | 0.163 | | | 0.169 |
| | CIPSI | 0.109 | 8.464 | 0.167 | 0.175 | 0.171 | 0.169 |
| | exFCI | 0.106(1) | 8.464(2) | 0.165(1) | 0.173(1) | 0.169(0) | 0.161(1) |

TABLE VII. Dipole moments and excitation energies for $H_2CO$ at the CC and SCI levels computed in various basis sets. An estimate of the exFCI extrapolation error is reported in parentheses.

| | | $^1A_1$ | $^1A_2$ (Val, $n \to \pi^*$) | |
|---|---|---|---|---|
| Basis | Method | $\lVert\boldsymbol{\mu}^{\text{GS}}\rVert$ (D) | $\Delta E_{\text{vert}}$ (eV) | $\lVert\boldsymbol{\mu}^{\text{ES}}\rVert$ (D) |
| 6-31+G(d) | CCSD | 2.584 | 4.031 | 1.710 |
| | CCSDT | 2.529 | 4.011 | 1.649 |
| | CCSDTQ | 2.518 | 4.021 | 1.629 |
| | CCSDTQP | 2.517 | 4.023 | 1.627 |
| | CIPSI | 2.517 | 4.022 | 1.626 |
| | exFCI | 2.516(0) | 4.023(0) | 1.626(0) |
| aug-cc-pVDZ | CCSD | 2.427 | 4.020 | 1.397 |
| | CCSDT | 2.368 | 3.986 | 1.337 |
| | CCSDTQ | 2.356 | 3.997 | 1.319 |
| | CIPSI | 2.360 | 3.994 | 1.318 |
| | exFCI | 2.355(1) | 3.998(1) | 1.317(0) |
| aug-cc-pVTZ | CCSD | 2.457 | 4.013 | 1.416 |
| | CCSDT | 2.389 | 3.954 | 1.346 |
| | CIPSI | 2.394 | 3.955 | 1.326 |
| | exFCI | 2.384(5) | 3.968(3) | 1.325(2) |

TABLE VIII. Dipole moments and excitation energies for $H_2CS$ at the CC and SCI levels computed in various basis sets. An estimate of the exFCI extrapolation error is reported in parentheses.

| | | $^1A_1$ | $^1A_2$ (Val, $n \to \pi^*$) | |
|---|---|---|---|---|
| Basis | Method | $\lVert \boldsymbol{\mu}^{GS} \rVert$ (D) | $\Delta E_{vert}$ (eV) | $\lVert \boldsymbol{\mu}^{ES} \rVert$ (D) |
| 6-31+G(d) | CCSD | 1.747 | 2.302 | 0.933 |
| | CCSDT | 1.733 | 2.244 | 0.948 |
| | CCSDTQ | 1.720 | 2.246 | 0.919 |
| | CCSDTQP | 1.719 | 2.247 | 0.917 |
| | CIPSI | 1.721 | 2.245 | 0.915 |
| | exFCI | 1.719(1) | 2.247(0) | 0.915(0) |
| aug-cc-pVDZ | CCSD | 1.742 | 2.325 | 0.851 |
| | CCSDT | 1.716 | 2.253 | 0.870 |
| | CCSDTQ | 1.704 | 2.255 | 0.848 |
| | CIPSI | 1.712 | 2.249 | 0.845 |
| | exFCI | 1.702(1) | 2.256(1) | 0.843(1) |
| aug-cc-pVTZ | CCSD | 1.737 | 2.291 | 0.848 |
| | CCSDT | 1.706 | 2.207 | 0.865 |
| | CIPSI | 1.729 | 2.188 | 0.829 |
| | exFCI | 1.695(3) | 2.211(3) | 0.839(6) |

TABLE IX. Dipole moments and excitation energies for HNO at the CC and SCI levels computed in various basis sets. An estimate of the exFCI extrapolation error is reported in parentheses.

| | | $^1A'$ | $^1A''$ (Val, $n \to \pi^*$) | |
|---|---|---|---|---|
| Basis | Method | $\lVert \boldsymbol{\mu}^{GS} \rVert$ (D) | $\Delta E_{vert}$ (eV) | $\lVert \boldsymbol{\mu}^{ES} \rVert$ (D) |
| 6-31+G(d) | CCSD | 1.902 | 1.802 | 1.982 |
| | CCSDT | 1.876 | 1.796 | 1.948 |
| | CCSDTQ | 1.869 | 1.799 | 1.938 |
| | CCSDTQP | 1.868 | 1.800 | 1.937 |
| | CIPSI | 1.869 | 1.797 | 1.938 |
| | exFCI | 1.867(1) | 1.800(0) | 1.937(1) |
| aug-cc-pVDZ | CCSD | 1.701 | 1.779 | 1.719 |
| | CCSDT | 1.667 | 1.767 | 1.681 |
| | CCSDTQ | 1.658 | 1.770 | 1.670 |
| | CIPSI | 1.664 | 1.762 | 1.673 |
| | exFCI | 1.658(0) | 1.770(1) | 1.668(1) |
| aug-cc-pVTZ | CCSD | 1.722 | 1.756 | 1.727 |
| | CCSDT | 1.683 | 1.737 | 1.688 |
| | CIPSI | 1.693 | 1.722 | 1.682 |
| | exFCI | 1.676(1) | 1.744(4) | 1.675(3) |

TABLE X. Dipole moments, excitation energies, and oscillator strengths in the length (L), velocity (V), and mixed (LV) representation for FCH at the CC and SCI levels computed in various basis sets. An estimate of the exFCI extrapolation error is reported in parentheses.

| | | $^1A'$ | $^1A''$ | | | | |
|---|---|---|---|---|---|---|---|
| Basis | Method | $\|\mu^{GS}\|$ (D) | $\Delta E_{vert}$ (eV) | $f^L$ | $f^V$ | $f^{LV}$ | $\|\mu^{ES}\|$ (D) |
| 6-31+G(d) | CCSD | 1.572 | 2.581 | 0.009 | | | 1.316 |
| | CCSDT | 1.552 | 2.573 | 0.009 | | | 1.287 |
| | CCSDTQ | 1.549 | 2.577 | 0.009 | | | 1.282 |
| | CCSDTQP | 1.549 | 2.578 | 0.009 | | | 1.282 |
| | CIPSI | 1.550 | 2.576 | 0.009 | 0.044 | 0.020 | 1.280 |
| | exFCI | 1.550(1) | 2.578(0) | 0.009(0) | 0.044(0) | 0.020(0) | 1.280(0) |
| aug-cc-pVDZ | CCSD | 1.451 | 2.541 | 0.007 | | | 0.991 |
| | CCSDT | 1.430 | 2.529 | 0.006 | | | 0.970 |
| | CCSDTQ | 1.428 | 2.534 | 0.006 | | | 0.965 |
| | CIPSI | 1.433 | 2.527 | 0.006 | 0.010 | 0.008 | 0.964 |
| | exFCI | 1.429(1) | 2.534(0) | 0.006(0) | 0.010(0) | 0.008(0) | 0.962(0) |
| aug-cc-pVTZ | CCSD | 1.465 | 2.507 | 0.006 | | | 0.991 |
| | CCSDT | 1.441 | 2.493 | 0.006 | | | 0.969 |
| | CIPSI | 1.454 | 2.483 | 0.006 | 0.008 | 0.007 | 0.954 |
| | exFCI | 1.439(2) | 2.499(3) | 0.006(0) | 0.008(0) | 0.007(0) | 0.958(5) |

TABLE XI. Dipole moments, excitation energies, and oscillator strengths in the length (L), velocity (V), and mixed (LV) representation for $H_2CSi$ at the CC and SCI levels computed in various basis sets. An estimate of the exFCI extrapolation error is reported in parentheses.

| | | $^1A_1$ | $^1A_2$ | | $^1B_2$ | | | | |
|---|---|---|---|---|---|---|---|---|---|
| Basis | Method | $\|\mu^{GS}\|$ (D) | $\Delta E_{vert}$(eV) | $\|\mu^{ES}\|$ (D) | $\Delta E_{vert}$ (eV) | $f^L$ | $f^V$ | $f^{LV}$ | $\|\mu^{ES}\|$ (D) |
| 6-31+G(d) | CCSD | 0.091 | 2.254 | 1.845 | 3.966 | 0.045 | | | 0.080 |
| | CCSDT | 0.028 | 2.107 | 1.891 | 3.874 | 0.042 | | | 0.237 |
| | CCSDTQ | 0.019 | 2.101 | 1.909 | 3.876 | 0.042 | | | 0.256 |
| | CCSDTQP | 0.018 | 2.101 | 1.911 | 3.877 | 0.042 | | | 0.259 |
| | CIPSI | 0.017 | 2.100 | 1.915 | 3.876 | 0.042 | 0.041 | 0.042 | 0.258 |
| | exFCI | 0.017(1) | 2.101(0) | 1.914(1) | 3.877(0) | 0.042(0) | 0.041(0) | 0.042(0) | 0.258(0) |
| aug-cc-pVDZ | CCSD | 0.181 | 2.288 | 1.836 | 3.875 | 0.036 | | | 0.162 |
| | CCSDT | 0.115 | 2.146 | 1.889 | 3.795 | 0.034 | | | 0.005 |
| | CCSDTQ | 0.105 | 2.140 | 1.905 | 3.798 | 0.034 | | | 0.012 |
| | CIPSI | 0.103 | 2.129 | 1.925 | 3.793 | 0.034 | 0.032 | 0.033 | 0.018 |
| | exFCI | 0.101(4) | 2.139(1) | 1.912(5) | 3.800(1) | 0.034(0) | 0.031(0) | 0.033(0) | 0.012(1) |
| aug-cc-pVTZ | CCSD | 0.235 | 2.286 | 1.851 | 3.877 | 0.036 | | | 0.161 |
| | CCSDT | 0.153 | 2.128 | 1.905 | 3.779 | 0.033 | | | 0.018 |
| | CIPSI | 0.140 | 2.102 | 1.958 | 3.773 | 0.035 | 0.033 | 0.034 | 0.050 |
| | exFCI | 0.137(3) | 2.117(1) | 1.933(1) | 3.781(1) | 0.034(0) | 0.032(0) | 0.033(0) | 0.041(1) |

TABLE XII. Statistical measures associated with the errors (with respect to exFCI) of ground-state (GS) and excited-state (ES) dipole moments computed at the CCSD, CCSDT, and CCSDTQ levels in the 6-31+G(d) basis.

| Method | State | # state | MSE | MAE | SDE | RMSE | Max (+) | Max (−) |
|---|---|---|---|---|---|---|---|---|
| CCSD | All | 11 | $1.5 \times 10^{-2}$ | $6.0 \times 10^{-2}$ | $7.2 \times 10^{-2}$ | $7.3 \times 10^{-2}$ | $8.3 \times 10^{-2}$ | $-1.8 \times 10^{-1}$ |
| CCSD | GS | 5 | $4.5 \times 10^{-2}$ | $4.5 \times 10^{-2}$ | $2.1 \times 10^{-2}$ | $5.0 \times 10^{-2}$ | $7.3 \times 10^{-2}$ | 0.0 |
| CCSD | ES | 6 | $-1.1 \times 10^{-2}$ | $7.1 \times 10^{-2}$ | $8.8 \times 10^{-2}$ | $8.8 \times 10^{-2}$ | $8.3 \times 10^{-2}$ | $-1.8 \times 10^{-1}$ |
| CCSDT | All | 11 | $7.0 \times 10^{-3}$ | $1.5 \times 10^{-2}$ | $1.6 \times 10^{-2}$ | $1.7 \times 10^{-2}$ | $3.3 \times 10^{-2}$ | $-2.4 \times 10^{-2}$ |
| CCSDT | GS | 5 | $9.9 \times 10^{-3}$ | $9.9 \times 10^{-3}$ | $4.1 \times 10^{-3}$ | $1.1 \times 10^{-2}$ | $1.4 \times 10^{-2}$ | 0.0 |
| CCSDT | ES | 6 | $4.7 \times 10^{-3}$ | $2.0 \times 10^{-2}$ | $2.1 \times 10^{-2}$ | $2.1 \times 10^{-2}$ | $3.3 \times 10^{-2}$ | $-2.4 \times 10^{-2}$ |
| CCSDTQ | All | 11 | $8.5 \times 10^{-4}$ | $2.3 \times 10^{-3}$ | $2.5 \times 10^{-3}$ | $2.7 \times 10^{-3}$ | $4.0 \times 10^{-3}$ | $-5.5 \times 10^{-3}$ |
| CCSDTQ | GS | 5 | $1.3 \times 10^{-3}$ | $1.4 \times 10^{-3}$ | $8.6 \times 10^{-4}$ | $1.6 \times 10^{-3}$ | $2.3 \times 10^{-3}$ | $-1.8 \times 10^{-4}$ |
| CCSDTQ | ES | 6 | $4.5 \times 10^{-4}$ | $3.0 \times 10^{-3}$ | $3.3 \times 10^{-3}$ | $3.3 \times 10^{-3}$ | $4.0 \times 10^{-3}$ | $-5.5 \times 10^{-3}$ |

TABLE XIII. Statistical measures associated with the errors (with respect to exFCI) of ground-state (GS) and excited-state (ES) dipole moments computed at the CCSD, CCSDT, and CCSDTQ levels in the aug-cc-pVDZ basis.

| Method | State | # state | MSE | MAE | SDE | RMSE | Max (+) | Max (−) |
|---|---|---|---|---|---|---|---|---|
| CCSD | All | 26 | $1.8 \times 10^{-2}$ | $4.6 \times 10^{-2}$ | $5.3 \times 10^{-2}$ | $5.6 \times 10^{-2}$ | $1.5 \times 10^{-1}$ | $-7.5 \times 10^{-2}$ |
| CCSD | GS | 11 | $2.3 \times 10^{-2}$ | $3.7 \times 10^{-2}$ | $3.7 \times 10^{-2}$ | $4.3 \times 10^{-2}$ | $8.0 \times 10^{-2}$ | $-5.4 \times 10^{-2}$ |
| CCSD | ES | 15 | $1.5 \times 10^{-2}$ | $5.2 \times 10^{-2}$ | $6.1 \times 10^{-2}$ | $6.3 \times 10^{-2}$ | $1.5 \times 10^{-1}$ | $-7.5 \times 10^{-2}$ |
| CCSDT | All | 26 | $5.2 \times 10^{-3}$ | $8.9 \times 10^{-3}$ | $1.0 \times 10^{-2}$ | $1.1 \times 10^{-2}$ | $2.7 \times 10^{-2}$ | $-2.3 \times 10^{-2}$ |
| CCSDT | GS | 11 | $4.0 \times 10^{-3}$ | $6.1 \times 10^{-3}$ | $7.4 \times 10^{-3}$ | $8.4 \times 10^{-3}$ | $1.4 \times 10^{-2}$ | $-1.1 \times 10^{-2}$ |
| CCSDT | ES | 15 | $6.1 \times 10^{-3}$ | $1.1 \times 10^{-2}$ | $1.2 \times 10^{-2}$ | $1.3 \times 10^{-2}$ | $2.7 \times 10^{-2}$ | $-2.3 \times 10^{-2}$ |
| CCSDTQ | All | 26 | $9.4 \times 10^{-4}$ | $1.8 \times 10^{-3}$ | $2.2 \times 10^{-3}$ | $2.4 \times 10^{-3}$ | $4.7 \times 10^{-3}$ | $-6.3 \times 10^{-3}$ |
| CCSDTQ | GS | 11 | $4.0 \times 10^{-4}$ | $1.1 \times 10^{-3}$ | $1.6 \times 10^{-3}$ | $1.6 \times 10^{-3}$ | $3.8 \times 10^{-3}$ | $-2.4 \times 10^{-3}$ |
| CCSDTQ | ES | 15 | $1.3 \times 10^{-3}$ | $2.2 \times 10^{-3}$ | $2.5 \times 10^{-3}$ | $2.8 \times 10^{-3}$ | $4.7 \times 10^{-3}$ | $-6.3 \times 10^{-3}$ |

TABLE XIV. Statistical measures associated with the errors (with respect to exFCI) of ground-state (GS) and excited-state (ES) dipole moments computed at the CCSD, CCSDT, and CCSDTQ levels in the aug-cc-pVTZ basis.

| Method | State | # state | MSE | MAE | SDE | RMSE | Max (+) | Max (−) |
|---|---|---|---|---|---|---|---|---|
| CCSD | All | 26 | $1.7 \times 10^{-2}$ | $4.5 \times 10^{-2}$ | $5.3 \times 10^{-2}$ | $5.6 \times 10^{-2}$ | $1.2 \times 10^{-1}$ | $-8.2 \times 10^{-2}$ |
| CCSD | GS | 11 | $2.4 \times 10^{-2}$ | $4.1 \times 10^{-2}$ | $4.2 \times 10^{-2}$ | $4.9 \times 10^{-2}$ | $9.8 \times 10^{-2}$ | $-6.5 \times 10^{-2}$ |
| CCSD | ES | 15 | $1.3 \times 10^{-2}$ | $4.8 \times 10^{-2}$ | $5.9 \times 10^{-2}$ | $6.0 \times 10^{-2}$ | $1.2 \times 10^{-1}$ | $-8.2 \times 10^{-2}$ |
| CCSDT | All | 26 | $4.0 \times 10^{-3}$ | $9.2 \times 10^{-3}$ | $1.1 \times 10^{-2}$ | $1.2 \times 10^{-2}$ | $2.6 \times 10^{-2}$ | $-2.8 \times 10^{-2}$ |
| CCSDT | GS | 11 | $3.2 \times 10^{-3}$ | $5.5 \times 10^{-3}$ | $7.0 \times 10^{-3}$ | $7.7 \times 10^{-3}$ | $1.7 \times 10^{-2}$ | $-1.2 \times 10^{-2}$ |
| CCSDT | ES | 15 | $4.6 \times 10^{-3}$ | $1.2 \times 10^{-2}$ | $1.4 \times 10^{-2}$ | $1.5 \times 10^{-2}$ | $2.6 \times 10^{-2}$ | $-2.8 \times 10^{-2}$ |
| CCSDTQ | All | 15 | $8.4 \times 10^{-4}$ | $1.4 \times 10^{-3}$ | $2.0 \times 10^{-3}$ | $2.2 \times 10^{-3}$ | $5.3 \times 10^{-3}$ | $-2.9 \times 10^{-3}$ |
| CCSDTQ | GS | 6 | $-3.8 \times 10^{-4}$ | $6.4 \times 10^{-4}$ | $1.1 \times 10^{-3}$ | $1.2 \times 10^{-3}$ | $4.3 \times 10^{-4}$ | $-2.9 \times 10^{-3}$ |
| CCSDTQ | ES | 9 | $1.7 \times 10^{-3}$ | $1.8 \times 10^{-3}$ | $2.0 \times 10^{-3}$ | $2.6 \times 10^{-3}$ | $5.3 \times 10^{-3}$ | $-4.0 \times 10^{-4}$ |

TABLE XV. Statistical measures associated with the errors (with respect to exFCI) of ground-state (GS) and excited-state (ES) dipole moments computed at the CCSD, CCSDT, and CCSDTQ levels in the aug-cc-pVQZ basis.

| Method | State | # state | MSE | MAE | SDE | RMSE | Max (+) | Max (−) |
|---|---|---|---|---|---|---|---|---|
| CCSD | All | 15 | $-4.4 \times 10^{-3}$ | $3.3 \times 10^{-2}$ | $4.4 \times 10^{-2}$ | $4.4 \times 10^{-2}$ | $1.0 \times 10^{-1}$ | $-7.4 \times 10^{-2}$ |
| CCSD | GS | 6 | $-3.3 \times 10^{-3}$ | $2.9 \times 10^{-2}$ | $3.4 \times 10^{-2}$ | $3.4 \times 10^{-2}$ | $2.6 \times 10^{-2}$ | $-6.6 \times 10^{-2}$ |
| CCSD | ES | 9 | $-5.2 \times 10^{-3}$ | $3.6 \times 10^{-2}$ | $4.9 \times 10^{-2}$ | $5.0 \times 10^{-2}$ | $1.0 \times 10^{-1}$ | $-7.4 \times 10^{-2}$ |
| CCSDT | All | 15 | $2.5 \times 10^{-3}$ | $4.8 \times 10^{-3}$ | $5.5 \times 10^{-3}$ | $6.1 \times 10^{-3}$ | $1.2 \times 10^{-2}$ | $-1.2 \times 10^{-2}$ |
| CCSDT | GS | 6 | $-1.1 \times 10^{-3}$ | $3.2 \times 10^{-3}$ | $4.9 \times 10^{-3}$ | $5.0 \times 10^{-3}$ | $2.1 \times 10^{-3}$ | $-1.2 \times 10^{-2}$ |
| CCSDT | ES | 9 | $4.9 \times 10^{-3}$ | $5.9 \times 10^{-3}$ | $4.6 \times 10^{-3}$ | $6.7 \times 10^{-3}$ | $1.2 \times 10^{-2}$ | $-3.3 \times 10^{-3}$ |

TABLE XVI. Statistical measures associated with the errors (with respect to exFCI) of the oscillator strengths computed in the length representation at the CCSD, CCSDT, and CCSDTQ levels in the 6-31+G(d) basis.

| Method | State | # state | MSE | MAE | SDE | RMSE | Max (+) | Max (−) |
|---|---|---|---|---|---|---|---|---|
| 6-31+G(d) | CCSD | 2 | $1.4 \times 10^{-3}$ | $1.4 \times 10^{-3}$ | $1.2 \times 10^{-3}$ | $1.9 \times 10^{-3}$ | $2.6 \times 10^{-3}$ | 0.0 |
| 6-31+G(d) | CCSDT | 2 | $-2.0 \times 10^{-4}$ | $2.0 \times 10^{-4}$ | $1.7 \times 10^{-4}$ | $2.6 \times 10^{-4}$ | 0.0 | $-3.6 \times 10^{-4}$ |
| 6-31+G(d) | CCSDTQ | 2 | $-3.3 \times 10^{-5}$ | $3.3 \times 10^{-5}$ | $2.9 \times 10^{-5}$ | $4.4 \times 10^{-5}$ | 0.0 | $-6.1 \times 10^{-5}$ |

TABLE XVII. Statistical measures associated with the errors (with respect to exFCI) of the oscillator strengths computed in the length representation at the CCSD, CCSDT, and CCSDTQ levels in the aug-cc-pVDZ basis.

| Method | State | # state | MSE | MAE | SDE | RMSE | Max (+) | Max (−) |
|---|---|---|---|---|---|---|---|---|
| aug-cc-pVDZ | CCSD | 9 | $1.5 \times 10^{-4}$ | $2.3 \times 10^{-3}$ | $3.1 \times 10^{-3}$ | $3.1 \times 10^{-3}$ | $4.7 \times 10^{-3}$ | $-7.2 \times 10^{-3}$ |
| aug-cc-pVDZ | CCSDT | 9 | $-1.4 \times 10^{-4}$ | $4.0 \times 10^{-4}$ | $5.6 \times 10^{-4}$ | $5.8 \times 10^{-4}$ | $6.8 \times 10^{-4}$ | $-1.4 \times 10^{-3}$ |
| aug-cc-pVDZ | CCSDTQ | 9 | $-5.0 \times 10^{-5}$ | $8.2 \times 10^{-5}$ | $1.3 \times 10^{-4}$ | $1.4 \times 10^{-4}$ | $8.9 \times 10^{-5}$ | $-3.8 \times 10^{-4}$ |

TABLE XVIII. Statistical measures associated with the errors (with respect to exFCI) of the oscillator strengths computed in the length representation at the CCSD, CCSDT, and CCSDTQ levels in the aug-cc-pVTZ basis.

| Method | State | # state | MSE | MAE | SDE | RMSE | Max (+) | Max (−) |
|---|---|---|---|---|---|---|---|---|
| aug-cc-pVTZ | CCSD | 9 | $6.5 \times 10^{-4}$ | $2.5 \times 10^{-3}$ | $3.2 \times 10^{-3}$ | $3.3 \times 10^{-3}$ | $7.0 \times 10^{-3}$ | $-5.3 \times 10^{-3}$ |
| aug-cc-pVTZ | CCSDT | 9 | $-1.5 \times 10^{-4}$ | $3.9 \times 10^{-4}$ | $6.0 \times 10^{-4}$ | $6.1 \times 10^{-4}$ | $4.9 \times 10^{-4}$ | $-1.7 \times 10^{-3}$ |
| aug-cc-pVTZ | CCSDTQ | 7 | $-3.9 \times 10^{-5}$ | $6.4 \times 10^{-5}$ | $1.2 \times 10^{-4}$ | $1.3 \times 10^{-4}$ | $5.3 \times 10^{-5}$ | $-3.3 \times 10^{-4}$ |

TABLE XIX. Statistical measures associated with the errors (with respect to exFCI) of the oscillator strengths computed in the length representation at the CCSD, CCSDT, and CCSDTQ levels in the aug-cc-pVQZ basis.

| Method | State | # state | MSE | MAE | SDE | RMSE | Max (+) | Max (−) |
|---|---|---|---|---|---|---|---|---|
| aug-cc-pVQZ | CCSD | 7 | $4.8 \times 10^{-4}$ | $2.8 \times 10^{-3}$ | $3.5 \times 10^{-3}$ | $3.5 \times 10^{-3}$ | $7.1 \times 10^{-3}$ | $-5.0 \times 10^{-3}$ |
| aug-cc-pVQZ | CCSDT | 7 | $-1.7 \times 10^{-4}$ | $5.1 \times 10^{-4}$ | $7.6 \times 10^{-4}$ | $7.8 \times 10^{-4}$ | $4.3 \times 10^{-4}$ | $-1.9 \times 10^{-3}$ |
